# Supplementary material for: Parasitic Photon-Pair Suppression via Photonic Stop-Band Engineering
Source: arXiv:1609.00106 source file (2017-03-06)
Supplement: Supplementary file 1 [file dual-pumpSFWM_SuppInfo.pdf]

# Supplementary Materials: Parasitic photon-pair suppression via photonic stop-band engineering

L. G. Helt,<sup>1</sup> Agata M. Brańczyk,<sup>2</sup> Marco Liscidini,<sup>3</sup> and M. J. Steel<sup>1</sup>

<sup>1</sup>*Centre for Ultrahigh bandwidth Devices for Optical Systems (CUDOS),  
MQ Photonics Research Centre, QSciTech Research Centre,*

*Department of Physics and Astronomy,  
Macquarie University, NSW 2109, Australia*

<sup>2</sup>*Perimeter Institute for Theoretical Physics,  
Waterloo, Ontario, N2L 2Y5, Canada*

<sup>3</sup>*Dipartimento di Fisica, Università degli Studi di Pavia, via Bassi 6, Pavia, Italy*

Here we derive the longitudinal field distributions  $f_{a\omega}^{\text{in(out)}}(z)$  for the asymptotic-in and -out fields in a Bragg grating. These functions are used in the main text to evaluate the generalized phase-matching function  $J_{ab}(\omega_1, \omega_2, \omega_3, \omega_4)$ . Following [1], we define the longitudinal distribution of an asymptotic-in field, consisting of forward-travelling  $f_{a\omega}^+(z)$  and backward-travelling  $f_{a\omega}^-(z)$  components

$$f_{a\omega}^{\text{in}}(z) = f_{a\omega}^+(z) e^{ik_a(\omega)z} + f_{a\omega}^-(z) e^{-ik_a(\omega)z}, \quad (1)$$

as satisfying the stationary scalar wave equation

$$\left[ \frac{d^2}{dz^2} + \frac{\omega^2 \varepsilon_a(z)}{c^2} \right] f_{a\omega}^{\text{in}}(z) = 0, \quad (2)$$

subject to the boundary conditions

$$\begin{aligned} f_{a\omega}^+(0) &= 1, \\ f_{a\omega}^-(L) &= 0. \end{aligned} \quad (3)$$

Making the slowly-varying envelope approximation to neglect second derivatives of  $F_{a\omega}^+(z)$  and  $F_{a\omega}^-(z)$ , and taking the grating to be defined by the perturbation

$$\begin{aligned} \varepsilon_a(z) &= [\bar{n}_a(\omega) + \Delta n \cos(2k_a(\omega_B)z)]^2 \\ &\approx \bar{n}_a^2(\omega) + 2n_a(\omega) \Delta n \cos(2k_a(\omega_B)z), \end{aligned} \quad (4)$$

we find that (2) reduces to

$$\begin{aligned} &\left[ i \frac{df_{a\omega}^+(z)}{dz} + 2\kappa \cos(2k_a(\omega_B)z) f_{a\omega}^+(z) \right] e^{ik_a(\omega)z} \\ &+ \left[ -i \frac{df_{a\omega}^-(z)}{dz} + 2\kappa \cos(2k_a(\omega_B)z) f_{a\omega}^-(z) \right] e^{-ik_a(\omega)z} = 0, \end{aligned} \quad (5)$$

where we have defined

$$k_a(\omega) = \frac{\omega \bar{n}_a}{c}, \quad (6)$$

and

$$\kappa = \frac{\omega^2 n_a(\omega) \Delta n}{2c^2 k_a(\omega)} = \frac{\pi \Delta n}{\lambda}, \quad (7)$$

as in the main text. Finally, expanding

$$\cos(2k_a(\omega_B)z) = (e^{2ik_a(\omega_B)z} + e^{-2ik_a(\omega_B)z})/2, \quad (8)$$

we find that the effect of the perturbation (4) is to couple forward and backward propagating components

$$\begin{aligned}
& i \frac{\partial f_{a\omega}^+(z)}{\partial z} + \kappa e^{-2i[k_a(\omega) - k_a(\omega_B)]z} f_{a\omega}^-(z) \\
& - i \frac{\partial f_{a\omega}^-(z)}{\partial z} + \kappa e^{2i[k_a(\omega) - k_a(\omega_B)]z} f_{a\omega}^+(z) \\
& + \text{rapidly oscillating terms} = 0.
\end{aligned} \tag{9}$$

For this equation to hold true, each line must vanish identically, and so  $f_{a\omega}^{\text{in}}(z)$  is defined by the solutions of the coupled equations

$$\begin{aligned}
& i \frac{\partial f_{a\omega}^+(z)}{\partial z} + \kappa e^{-2i[k_a(\omega) - k_a(\omega_B)]z} f_{a\omega}^-(z) = 0 \\
& - i \frac{\partial f_{a\omega}^-(z)}{\partial z} + \kappa e^{2i[k_a(\omega) - k_a(\omega_B)]z} f_{a\omega}^+(z) = 0,
\end{aligned} \tag{10}$$

subject to the boundary conditions (3). These equations have solutions

$$\begin{aligned}
f_{a\omega}^+(z) &= \frac{e^{-i\delta_{a\omega}z} \{ \xi_{a\omega} \cosh[\xi_{a\omega}(L-z)] - i\delta_{a\omega} \sinh[\xi_{a\omega}(L-z)] \}}{\xi_{a\omega} \cosh(\xi_{a\omega}L) - i\delta_{a\omega} \sinh(\xi_{a\omega}L)}, \\
f_{a\omega}^-(z) &= i \frac{e^{i\delta_{a\omega}z} \kappa \sinh[\xi_{a\omega}(L-z)]}{\xi_{a\omega} \cosh(\xi_{a\omega}L) - i\delta_{a\omega} \sinh(\xi_{a\omega}L)},
\end{aligned} \tag{11}$$

where, as in the main text,  $\xi_{a\omega} = \sqrt{\kappa^2 - \delta_{a\omega}^2}$ ,  $\delta_{a\omega} = k_a(\omega) - k_a(\omega_B)$ . Returning to (1), we see that we can write the full longitudinal distribution of the asymptotic-in field as

$$f_{a\omega}^{\text{in}}(z) = F_{a\omega}^+(z) e^{ik_a(\omega_B)z} + F_{a\omega}^-(z) e^{-ik_a(\omega_B)z}, \tag{12}$$

where we have defined

$$\begin{aligned}
F_{a\omega}^+(z) &= \frac{\xi_{a\omega} \cosh[\xi_{a\omega}(L-z)] - i\delta_{a\omega} \sinh[\xi_{a\omega}(L-z)]}{\xi_{a\omega} \cosh(\xi_{a\omega}L) - i\delta_{a\omega} \sinh(\xi_{a\omega}L)}, \\
F_{a\omega}^-(z) &= i \frac{\kappa \sinh[\xi_{a\omega}(L-z)]}{\xi_{a\omega} \cosh(\xi_{a\omega}L) - i\delta_{a\omega} \sinh(\xi_{a\omega}L)}.
\end{aligned} \tag{13}$$

Additionally, the longitudinal distribution of an asymptotic-out field can be written

$$f_{a\omega}^{\text{out}}(z) = g_{a\omega}^+(z) e^{ik_a(\omega)z} + g_{a\omega}^-(z) e^{-ik_a(\omega)z}, \tag{14}$$

defined by solutions of the coupled mode equations

$$\begin{aligned}
& i \frac{\partial g_{a\omega}^+(z)}{\partial z} + \kappa e^{-2i[k_a(\omega) - k_a(\omega_B)]z} g_{a\omega}^-(z) = 0 \\
& - i \frac{\partial g_{a\omega}^-(z)}{\partial z} + \kappa e^{2i[k_a(\omega) - k_a(\omega_B)]z} g_{a\omega}^+(z) = 0,
\end{aligned} \tag{15}$$

subject to the boundary conditions

$$\begin{aligned} g_{a\omega}^+(L) &= 1, \\ g_{a\omega}^-(0) &= 0. \end{aligned} \tag{16}$$

These equations have solutions

$$\begin{aligned} g_{a\omega}^+(z) &= \frac{e^{i\delta_{a\omega}(L-z)} [\xi_{a\omega} \cosh(\xi_{a\omega} z) + i\delta_{a\omega} \sinh(\xi_{a\omega} z)]}{\xi_{a\omega} \cosh(\xi_{a\omega} L) - i\delta_{a\omega} \sinh(\xi_{a\omega} L)}, \\ g_{a\omega}^-(z) &= \frac{e^{i\delta_{a\omega}(L+z)} \kappa \sinh[\xi_{a\omega} a]}{i\xi_{a\omega} \cosh(\xi_{a\omega} L) - \delta_{a\omega} \sinh(\xi_{a\omega} L)}, \end{aligned} \tag{17}$$

allowing us to write the full longitudinal distribution of the asymptotic-out field as

$$f_{a\omega}^{\text{out}}(z) = G_{a\omega}^+(z) e^{ik_a(\omega_B)z} + G_{a\omega}^-(z) e^{-ik_a(\omega_B)z}, \tag{18}$$

where we have defined

$$\begin{aligned} G_{a\omega}^+(z) &= \frac{[\xi_{a\omega} \cosh(\xi_{a\omega} z) + i\delta_{a\omega} \sinh(\xi_{a\omega} z)] e^{i\delta_{a\omega} L}}{\xi_{a\omega} \cosh(\xi_{a\omega} L) - i\delta_{a\omega} \sinh(\xi_{a\omega} L)}, \\ G_{a\omega}^-(z) &= \frac{\kappa \sinh(\xi_{a\omega} a) e^{i\delta_{a\omega} L}}{i\xi_{a\omega} \cosh(\xi_{a\omega} L) - \delta_{a\omega} \sinh(\xi_{a\omega} L)}, \end{aligned} \tag{19}$$

exactly as in Eqs. (8) of the main text.

---

[1] M. Liscidini, L. G. Helt, and J. E. Sipe, Phys. Rev. A **85**, 013833 (2012).
